# Supplementary material for: Relation between charging times and storage properties of nanoporous supercapacitors
Source: arXiv:2011.04575 source file (2021-05-19)
Supplement: Supplementary file 1 [file analytics.tex]

\section{Analytical derivation}
\subsection{Pressure}
The Gibbs-Duhem equation shows how the component chemical potentials relate to the pressure:
\begin{equation}
\label{eq:Gibbs-Duhem}
VdP=N_1d\mu_1+N_2d\mu_2
\end{equation}
After substitution of Gibbs-Duhem relation in terms of the average densities $\overline{\rho}_i=N_i/V$ the dynamic equation can be rewritten as follows
\begin{equation}
\partial_t (\overline{\rho}_1+\overline{\rho}_2)=D\beta\partial_x (\overline{\rho_1}\partial_x \mu_1+\overline{\rho_2}\partial_x \mu_2)=D\beta \partial_x^2 P(\overline{\rho}_1,\overline{\rho}_2) \nonumber
\end{equation}
The Helmholtz free energy can be rewritten as follows: 
\begin{align}
\label{eq:}
F=F_\text{id}+F_\text{hs}+F_\text{el}+k T\sum_i\int dr\rho_i(r)U_{C,i}(r)+ \nonumber 
\\
\sum_i A\int dz \rho_i(z)\left[U_{w,i}(z)+U_{w,i}(H-z)+Z_i e\psi(z,H)\right]
\end{align}
We denote the terms which depend on the $H$ explicitly as $U_{ext}(z,H)$, then
\begin{equation}
\rho_i(z)=\frac{\delta F}{\delta U_{ext}(z,H)}=\frac{\delta \Omega}{\delta U_{ext}(z,H)}
\end{equation}
The confined pressure in the open system is derived from the following volume derivative:
\begin{widetext}
\begin{align}
    \psi(z)=U_0+\frac{4\pi l_\text{B} z}{H}\int_0^H (H-z')\sum_{k=1}^n Z_k \rho_k(z')dz'
-4\pi l_\text{B}\int_0^z(z-z')\sum_{k=1}^n Z_k \rho_k(z')dz' 
%= \nonumber \\
%=U_0+2\pi l_B z H\int_0^1d\xi q(\xi)-4\pi l_\text{B}\int_0^z(z-z')\sum_{k=1}^n Z_k \rho_k(z')dz' \nonumber 
\\
\frac{d\psi(z,H)}{d H}=-\frac{4\pi l_B z}{H^2} \int_0^H dz' (H/2+H/2-z')q(z')+0+\frac{4\pi l_B z}{H}\int_0^Hdz'q(z')=-\frac{2\pi l_B z}{H}Q
\end{align}
\begin{align*}
P=-\frac{d\Omega}{d V}=-\sum_i\int_{0}^H dz \rho_i(z)\frac{d U_{ext}(z,H)}{d H}
=-\sum_i\int_{0}^H dz \rho_i(z)\frac{d}{d H} \left[ \theta(-z+d/2)+\theta(z-H+d/2)+Z_i e \psi(z,H)\right]= \nonumber\\
=
%\rho(d/2)-Z_i 4\pi l_B  e \int_{0}^Hz\rho_i(z)dz\left[-\frac{1}{H^2}\int_0^Hdz'(H/2+H/2-z')q(z')+\frac{1}{H}\int_{0}^Hdz'q(z')\right]=\rho(d/2)-\frac{2\pi l_B (-Q)}{H}\int_0^H dz z q(z)= \nonumber \\
\rho(d/2)+\frac{2\pi l_B Q}{H}\int_0^Hdz z\sum_i Z_i\rho_i(z)
=\rho(d/2)-\frac{Q}{2H}\int_0^H dz z \psi''(z) \nonumber \\
=\rho(d/2)-\frac{Q}{2H}\left[ H \psi'(H)-\int_0^Hdz\psi'(z)\right]=\rho(d/2)+\frac{Q}{2}\psi'(0)=\rho(d/2)-2\pi l_B \frac{Q^2}{2}
\end{align*}
\end{widetext}
The system of charge hard spheres exhibits the following pressure:
\begin{equation}
\label{eq:pressure}
\beta P= \rho_1(d/2)+\rho_2(d/2)-\frac{Q^2}{2\epsilon_0\epsilon k T}=\rho(d/2)-2\pi\frac{Q^{*2}\lambda_B}{d^4}
\end{equation}
\begin{equation}
\rho_i(d/2)=\rho_i^{(0)}\exp\left[-Z_i U_0^*+Z_i \pi\lambda_B Q^*-\beta \Delta\mu_i^{\text{exc}}|_{z=d/2}\right] \nonumber
\end{equation}

\subsection{Linearization near the final state}
In order to describe charging dynamics at the later stage, one can linearize the transport equations \eqref{eq:transport_average} near the final steady-state solution $\bar{\rho}_i (x, t) = \bar{\rho}^{f}_{i} + \bar{\rho}'_{i}$, $\bar{\rho}^{f}_{i}~=~const$ to get the system $\partial_t \bar{\rho}'_i - D_{ij} \partial_{xx} \bar{\rho}'_j = 0$ for the small corrections of densities $\rho'_i$ to the final steady-state solution. Here the matrix $D$ is given by
\begin{equation*}
D = \left.
\begin{pmatrix}
\bar{\rho}_1 \dfrac{\partial \mu_1}{\partial \bar{\rho}_1} & \bar{\rho}_1 \dfrac{\partial \mu_1}{\partial \bar{\rho}_2} \\
\bar{\rho}_2 \dfrac{\partial \mu_2}{\partial \bar{\rho}_1} & \bar{\rho}_2 \dfrac{\partial \mu_2}{\partial \bar{\rho}_2}
\end{pmatrix} \right|_{\bar{\rho}_i = \bar{\rho}^f_i}.
\end{equation*}

Using the Gibbs-Duhem relation \eqref{eq:Gibbs-Duhem} one can prove that the cross-derivatives of the chemical potentials with respect to average densities are equal
\begin{equation*}
\dfrac{\partial \mu_1}{\partial \bar{\rho}_2} = \dfrac{\partial \mu_2}{\partial \bar{\rho}_1}.
\end{equation*}
Utilizing the latter identity one can also show that the discriminant of the characteristic polynomial of the matrix $D$ is positive, the matrix has distinct real eigenvalues $\lambda_{1,2}$ and complete system of eigenvectors $\Omega$ and, thus, is diagonalizable $D = \Omega^{-1} \Lambda \Omega$, $\Lambda = \mathrm{diag} (\lambda_1, \lambda_2)$. Multiplication of the linearized equations by $\Omega$ gives the system of {\it decoupled} linear diffusion equations for linear combinations of corrections $\bar{\rho}'_i$. Since the boundary conditions for the corrections are essentially the same as for $\bar{\rho}_i$ (given value $\bar{\rho}'_i = 0$ at $x = 0$ and zero flux $\partial_x \bar{\rho}'_i = 0$ at $x = L$), the same is valid for those linear combinations. Accordingly, the TLM solution discussed above can be applied for both equations independently and it will result in two different timescales $\tau_{1,2}$ defined by the corresponding eigenvalues.

The eigenvalues $\lambda_{1,2}$ are given by
\begin{equation*}
\lambda_{1,2} = \dfrac{1}{2} \left(\mathrm{tr} D \pm \sqrt{(\mathrm{tr} D)^2 - 4 \mathrm{det} D}\right).
\end{equation*}

The ratio of the eigenvalues $\lambda$ is a function of the ratio $\mathrm{det} D / (\mathrm{tr} D)^2$ only. It can be shown that $\lambda \ll 1 \Leftrightarrow \mathrm{det} D / (\mathrm{tr} D)^2 \ll 1$. Furthermore, if the ideal gas contribution in \eqref{eq:pressure} is small compared to charge term, one can show that 
\begin{equation}
\label{eq:det_tr2}
\frac{\mathrm{det} D}{(\mathrm{tr} D)^2} = c (1 - c) \left(\frac{\mu}{(c + (1 - c) \mu)^2} - 1\right).
\end{equation}
Here 
\begin{equation*}
c = \frac{\bar{\rho}_1}{\bar{\rho}_1 + \bar{\rho}_2}, \quad \mu = \frac{\partial \mu_2}{\partial \bar{\rho}_2} / \frac{\partial \mu_1}{\partial \bar{\rho}_1}.
\end{equation*}
The expression \eqref{eq:det_tr2} has four zero-curves at $c-\mu$ plane: $c = 0$,  $c = 1$, $\mu = 1$ and $\mu = \mu^*(c)$. 

Accordingly, for large charges ($P \sim Q^2$) and low fractions of co-ions ($c \approx 1$) the ratio of the eigenvalues is small $\lambda \ll 1$ independent of chemical potential derivatives. It also may happen for certain very special conditions $\mu \approx 1$ and $\mu \approx \mu^*(c)$ (again, as long as $P \sim Q^2$).

\subsection{Calculation of the chemical potential derivatives}
Equations for the equilibrium distributions of densities in transverse direction may be written as
$\mu_i = \log \rho_i + G_i$ or equivalently as $\rho_i = \exp (\mu_i) F_i$, where $F_i = \exp (-G_i)$. Integrating over the pore width one can eliminate the chemical potentials and get the equations for density distributions in terms of average densities only
\begin{equation*}
\rho_i = \bar{\rho}_i \dfrac{F_i}{\bar{F_i}}, \quad \bar{F}_i = \int^1_0 dz \; F = \int^1_0 dz \; \exp(-G_i).
\end{equation*}
Differentiation of both sides of the equation with respect to the average densities and algebraic transformations give
\begin{gather*}
\bar{\rho}_i \dfrac{\partial \mu_i}{\partial \bar{\rho}_i} = 1 - \bar{\rho}_i \dfrac{\partial}{\partial \bar{\rho}_i} \log \bar{F}_i, \\
\bar{\rho}_i \dfrac{\partial \mu_i}{\partial \bar{\rho}_j} = - \bar{\rho}_i \dfrac{\partial}{\partial \bar{\rho}_j} \log \bar{F}_i, \quad j \neq i
\end{gather*}
\color{red} The question is can we somehow (saddle-point method?) estimate $\log \bar{F}_i$? Or show that
\begin{equation*}
\dfrac{\partial \mu_i}{\partial \bar{\rho}_i} \gg \dfrac{\partial \mu_i}{\partial \bar{\rho}_j}, \quad j \neq i?
\end{equation*}
If the latter is true, eigenvalues are simply diagonal elements.
\color{black}
